# Supplementary material for: Variational Schr\"odinger Diffusion Models
Source: arXiv:2405.04795 source file (2025-05-24)
Supplement: Supplementary file 1 [file B.appendix.tex]

\newpage

\subsection{Experimental Details}
\label{app:exp_details}
Flow matching 

\begin{equation*}
    u_t(x|z)=\frac{\sigma'_t(z)}{\sigma_t(z)}(x-\mu_t(z))+\mu_t'(z).
\end{equation*}

Gaussian Schrodinger bridge

\begin{equation*}
    d X_t = f_N(t, X_t)dt+g_t dW_t,
\end{equation*}
where
\begin{equation*}
    f_N(t, x)=S_t^T\Sigma_t^{-1}(x-\mu_t)+\dot{\mu}_t
\end{equation*}

Check the gradient of divergence in Tianrong's framework to see if we can directly use his framework but restrict the forward network to time-variant linear.

Three versions, full rank, diagonal, and ????

the reparametrization trick.

TO DO LIST:

\begin{itemize}
    \item \textcolor{red}{Given Gaussian data, show the result matches Gaussian SB.}
    \item \textcolor{red}{Comparision with flow matching. Conditional Flow Matching mentions about connections to SB.}
\end{itemize}

One key ref: Gaussian Schrodinger bridge. SB. Use a closed-form solution to show our result matching Gaussian SB given Gaussian data.

one helpful reference: Deep Variational Bayes Filters: Unsupervised Learning of State Space Models from Raw Data

One key reference: Stochastic Variational Inference.

The linear drift should be symmetric semi-positive definite $\bA_t$.

To achieve the symmetric target, we can learn B first and use $B+B^\intercal=A$.

To make sure it is semi-positive definite, we can apply the exponential transformation such that

If $A$ is symmetric, we can write $A=PDP^\intercal$
where $D$ is a diagonal matrix and $P$ is an orthogonal matrix. Then

$e^A = e^{PDP^\intercal}=Pe^D P^\intercal$

% import torch
% m = torch.nn.Linear(2, 2)
% input = torch.randn(3, 2)
% m(input)
% torch.matmul(m.weight, input.t()).t() + m.bias
% %%%%%%% symmetric matrix 
% sym_A = (m.weight + m.weight.t()) / 2
% torch.matmul(sym_A, input.t()).t() + m.bias
% %%%%%%% exponential of symmetric matrix
% exp_sym_A = torch.matrix_exp(sym_A)
% torch.matmul(exp_sym_A, input.t()).t() + m.bias

Connections to preconditioned XXXX.

\section{Others}

\textbf{parametrization}

\begin{itemize}
    \item Linear case: $\beta_t=\beta_{\min} + t(\bar\beta_{\max}-\bar\beta_{\min})$, we have $B_t=\int_0^t \beta_s \dd s=t\bar\beta_{\min} + \frac{t^2}{2}(\bar\beta_{\max}-\bar\beta_{\min})$
    \item Nonlinear case: $\beta_t=\beta_{\min} + t^{\alpha}(\bar\beta_{\max}-\bar\beta_{\min})$, $B_t=\int_0^t \beta_s \dd s=t\bar\beta_{\min} + \frac{t^{\alpha+1}}{\alpha+1}(\bar\beta_{\max}-\bar\beta_{\min})$.
\end{itemize}

Hyperparameters: parameterize orthogonal matrices by the Householder transform.

% The prior distribution may be standard Gaussian but rather has some covariance.

\textbf{Now we have a more general OU process where the coefficient is no longer a scaler but rather a matrix.}

% \Wei{whether to change the diffusion term in matrix form is still undecided.}

% \section{Divergence calculation based on linear SDE }
% \textcolor{blue}{Yu: I will fill details here.}

% The training algorithm in \citep{forward_backward_SDE} suffers from the calculation of the divergence through Jacobian matrix, which takes a large portion of computation and memory resources. 
% The back-propagation of the full Jacobian matrix scales quadratically w.r.t. the layer size,
% Our proposed method alleviate the problem by training the backward model based on DSM training, which only depends on first-order derivative.
% When training the forward model, while it still requires the calculation of the divergence, but it comes with analytical form based on linear SDE, which bypasses the back-propagation calculation using automatic differentiation frameworks.

\textbf{Normalizing Flows: An Introduction and Review
of Current Methods}

section 3 mentioned about 5 forms of the flows:
https://arxiv.org/pdf/1908.09257.pdf

3.2.1 a diagonal linear flow: L. Dinh, J. Sohl-Dickstein, and S. Bengio, “Density Estimation using Real NVP,” in ICLR, 2017.

3.2.2 Triangular: J. Tomczak and M. Welling, “Improving Variational AutoEncoders using convex combination linear Inverse Autoregressive Flow,” Benelearn, 2017.

3.2.3 Permutation and Orthogonal The expressiveness of triangular transformations.

3.2.4 Factorizations

3.2.5 Convolution

% , as such $\bP^{-1}$ is attainable via the $\text{triangular solver}$ in PyTorch.
